# Supplementary material for: FinFlier: Automating Graphical Overlays for Financial Visualizations with Knowledge-Grounding Large Language Model
Source: arXiv:2412.06821 source file (2024-12-05)
Supplement: Supplementary file 1 [file appendix_submit.tex]

% \documentclass[10pt,journal,compsoc]{IEEEtran}
% \usepackage{graphicx}
% \usepackage{etoolbox}
% \makeatletter
% \def\@xobeysp{\hspace{0pt}\mbox{ }\hspace{0pt}}
% \appto\verbatim@font{\hyphenchar\font`-\relax}
% \apptocmd\@sverb{\hspace*{0pt}}{}{}
% \makeatother
% \usepackage[justification=centering]{caption}

% \begin{document}

\appendices
\section{Binding Result Examples}\label{sec:appendix}
In this section, we display the binding result template through an example of the change pattern in GDP. The given text describes that the change in real GPD suffers a sharp decrease and then a rise. The subject \emph{change in real GDP} and two trend vocabularies: \emph{sharp decrease} and \emph{rise} are identified by our knowledge-grounding LLM and the following is its binding result.

{\small
\begin{verbatim}
Result:{
    "ObjectName": "change in real GDP",
    "DataName": "change in GDP",
    "Position": [["change in GDP", 7], ["change in GDP", 10]],
    "Trend": "sharp decrease",
    "Num": [Null],
    "Text": "the change in real GDP suffers a sharp decrease"},
{
    "ObjectName": "change in real GDP",
    "DataName": "change in GDP",
    "Position": [["change in GDP", 11], ["change in GDP", 14]],
    "Trend": "rise",
    "Num": [Null],
    "Text": "then a rise."}
Reason: "There is one object in text and data table: 'change in real GDP', which  corresponds
to 'change in GDP' column in the table. The trend for object 'change in real GDP' is 'sharp 
decrease', which corresponds to the column 'change in GDP' and from row 7 to row 10. The 
second trend for object 'change in real GDP' is 'rise', which corresponds to the column 'change in GDP' and from row 11 to row 14."
\end{verbatim}

\begin{verbatim}
Result: {
    "ObjectName": "active China-focused hedge funds",
    "DataName":"Active",
    "Position":[["Active",3],["Active",3]}],
    "Trend": "None",
    "Num": [669],
    "Text": "The number of active China-focused hedge funds has first reached 669."},
{
    "ObjectName": "funds launched",
    "DataName": "Launches",
    "Position":[["Launches",1], ["Launches",1]}],
    "Trend":"None",
    "Num":[5],
    "Text":"only five new funds launched this year as of June"},
{
    "ObjectName": "funds were liquidated",
    "DataName": "Liquidations",
    "Position":[["Liquidations",2], ["Liquidations",2]],
    "Trend":"None",
    "Num":[18],
    "Text":"Another 18 funds were liquidated"}
Reason: "There are three objects in text and data table: 'active China-focused hedge funds',
which corresponds to 'Active' column in the table, 'funds launched' corresponding to 'Launches'
column, and 'funds were liquidated' corresponds to 'Liquidations'. The numerical value for 
object 'active China-focused hedge funds' is 669, which corresponds to the column 'Active' 
and row 3. The numerical value for object 'funds launched' is 5, which corresponds to the 
column 'Launches' and row 1. The numerical value for object 'funds were liquidated' is 18, which corresponds to the column 'Liquidations' and row 2." 

\end{verbatim}}

\section{Narrative Examples}\label{sec:examplecom}
In this section, we present some narrative examples used in the user study.
For each narrative, the left figure shows the side-by-side interplay without linking; the middle one shows the side-by-side interplay with visual linking; and the right figure shows the \emph{FinFlier}'s generated layered charts.

\begin{figure}[h]
    \centering
    \includegraphics[width = 0.96\linewidth]{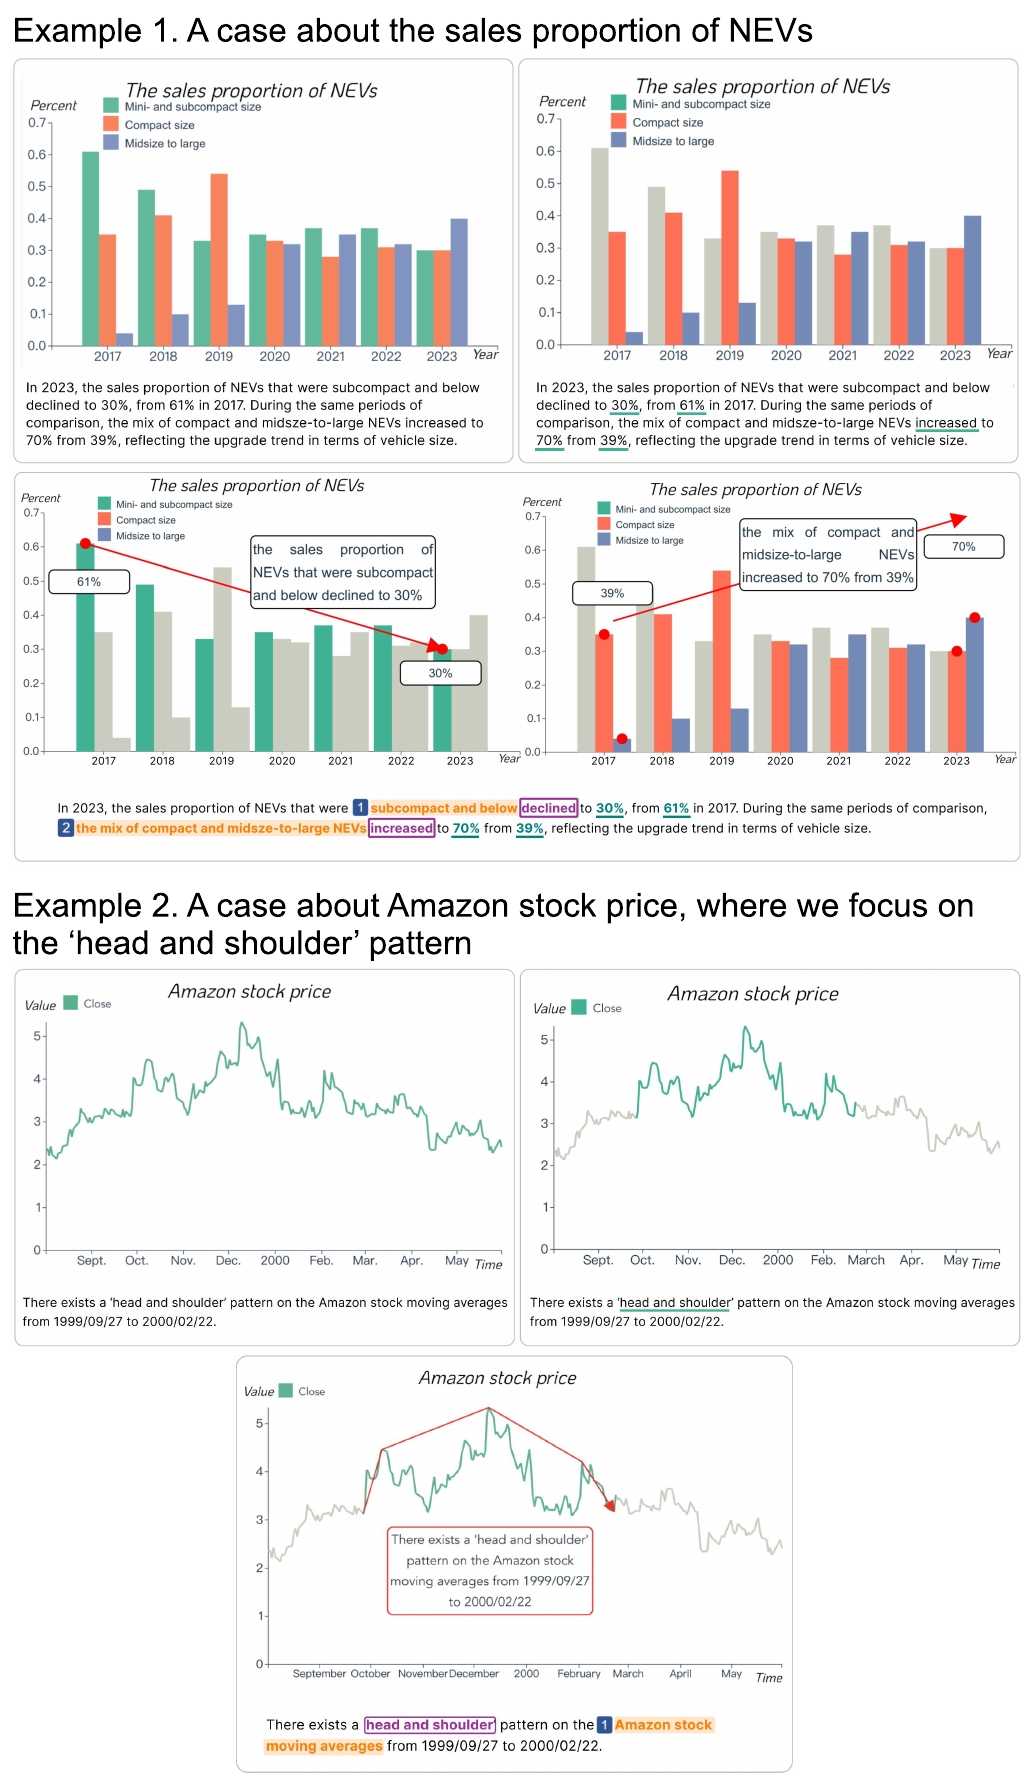}
\end{figure}

\begin{figure}[ht]
    \centering
    \includegraphics[width = 0.99\linewidth]{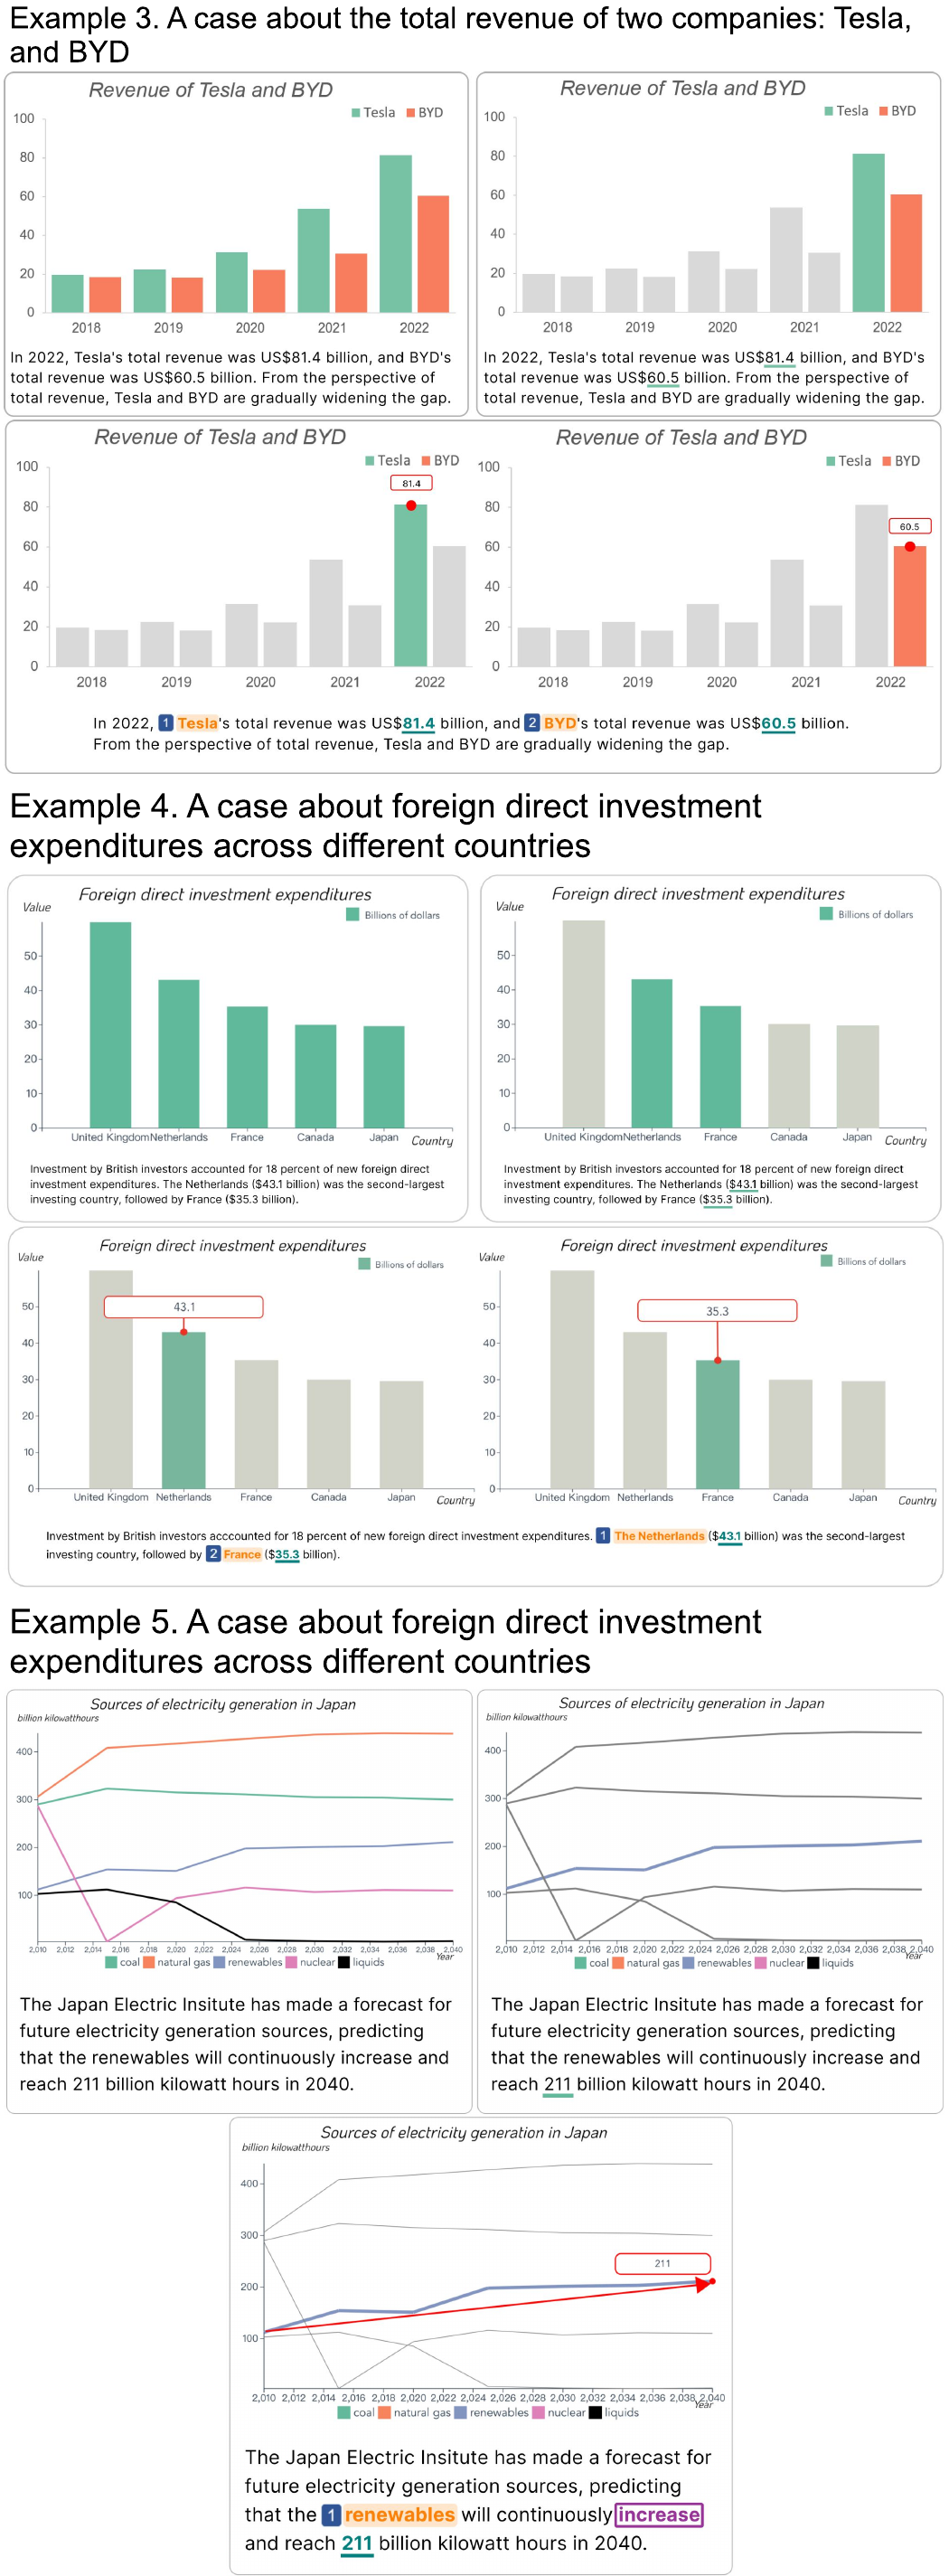}
\end{figure}

% \end{document}
